# Supplementary material for: In Search of a Data Transformation That Accelerates Neural Field Training
Source: arXiv:2311.17094 source file (2024-03-26)
Supplement: Supplementary file 1 [file LC_clic.tex]

\begin{figure*}[!t]
\centering
    % Row 1
    \begin{subfigure}[t]{0.32\linewidth}
        \centering
        \includegraphics[width=\linewidth]{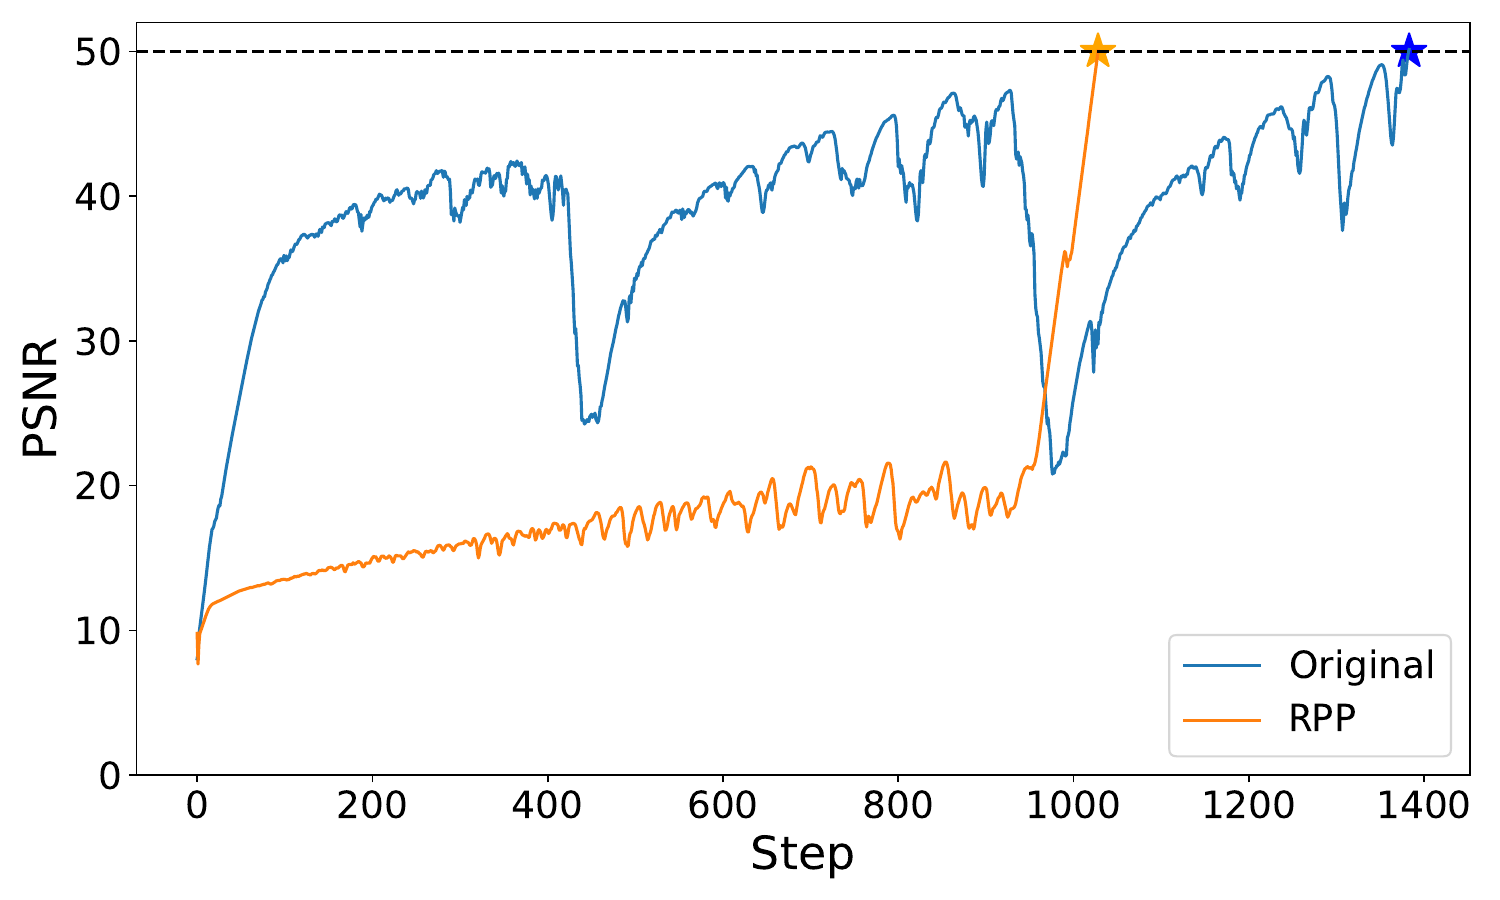}
        \captionsetup{skip=0pt}
        \caption{CLIC 01}
        \label{fig:lc_clic1}
    \end{subfigure}
    \hfill
    \begin{subfigure}[t]{0.32\linewidth}
        \centering
        \includegraphics[width=\linewidth]{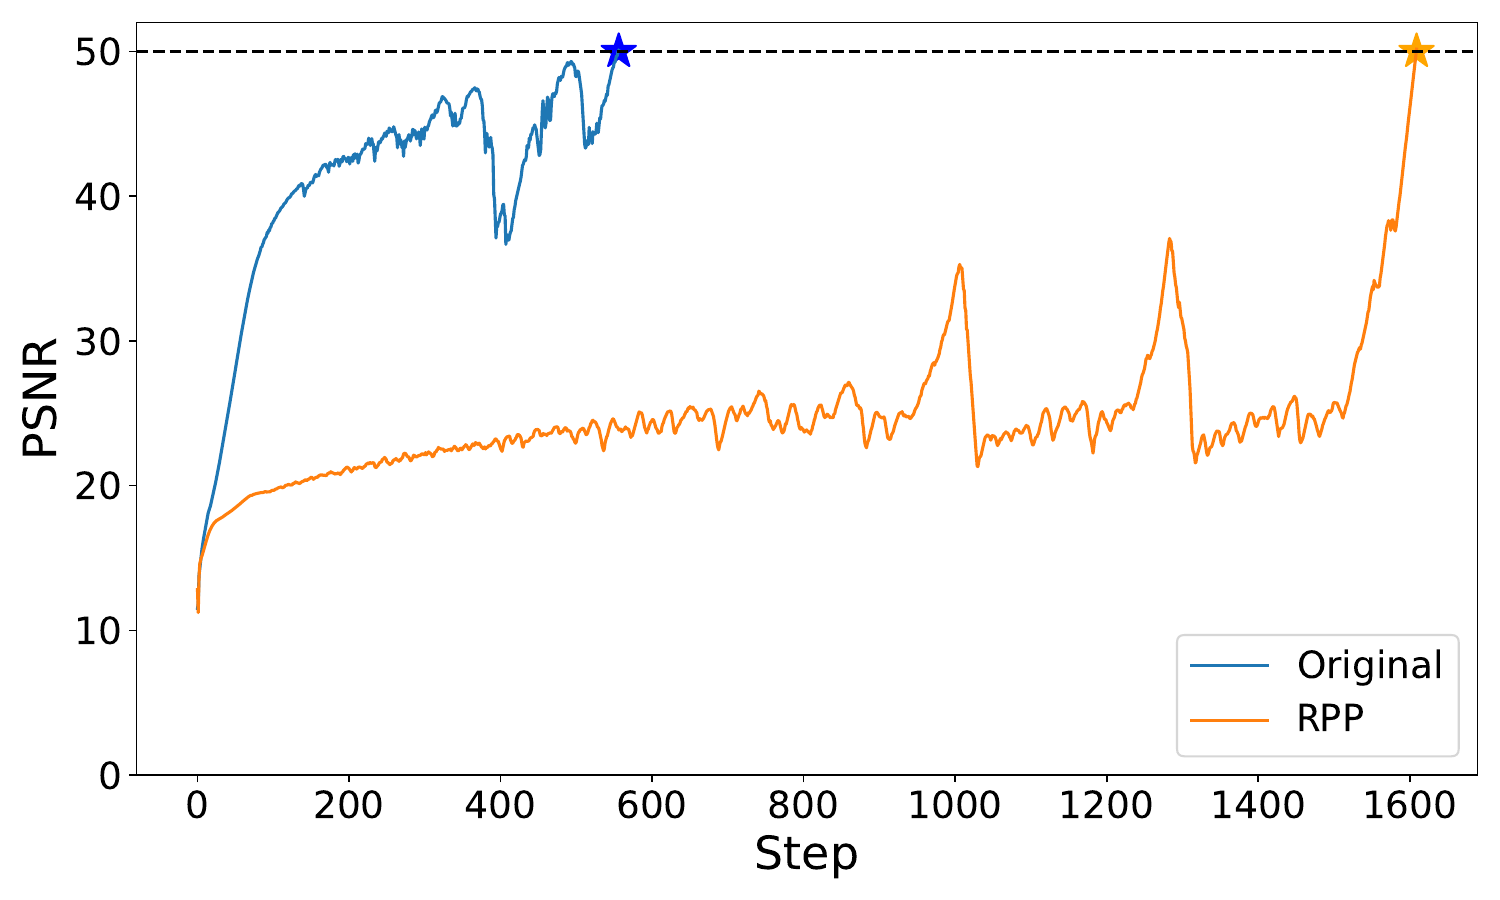}
        \captionsetup{skip=0pt}
        \caption{CLIC 02}
        \label{fig:lc_clic2}
    \end{subfigure}
    \hfill
    \begin{subfigure}[t]{0.32\linewidth}
        \centering
        \includegraphics[width=\linewidth]{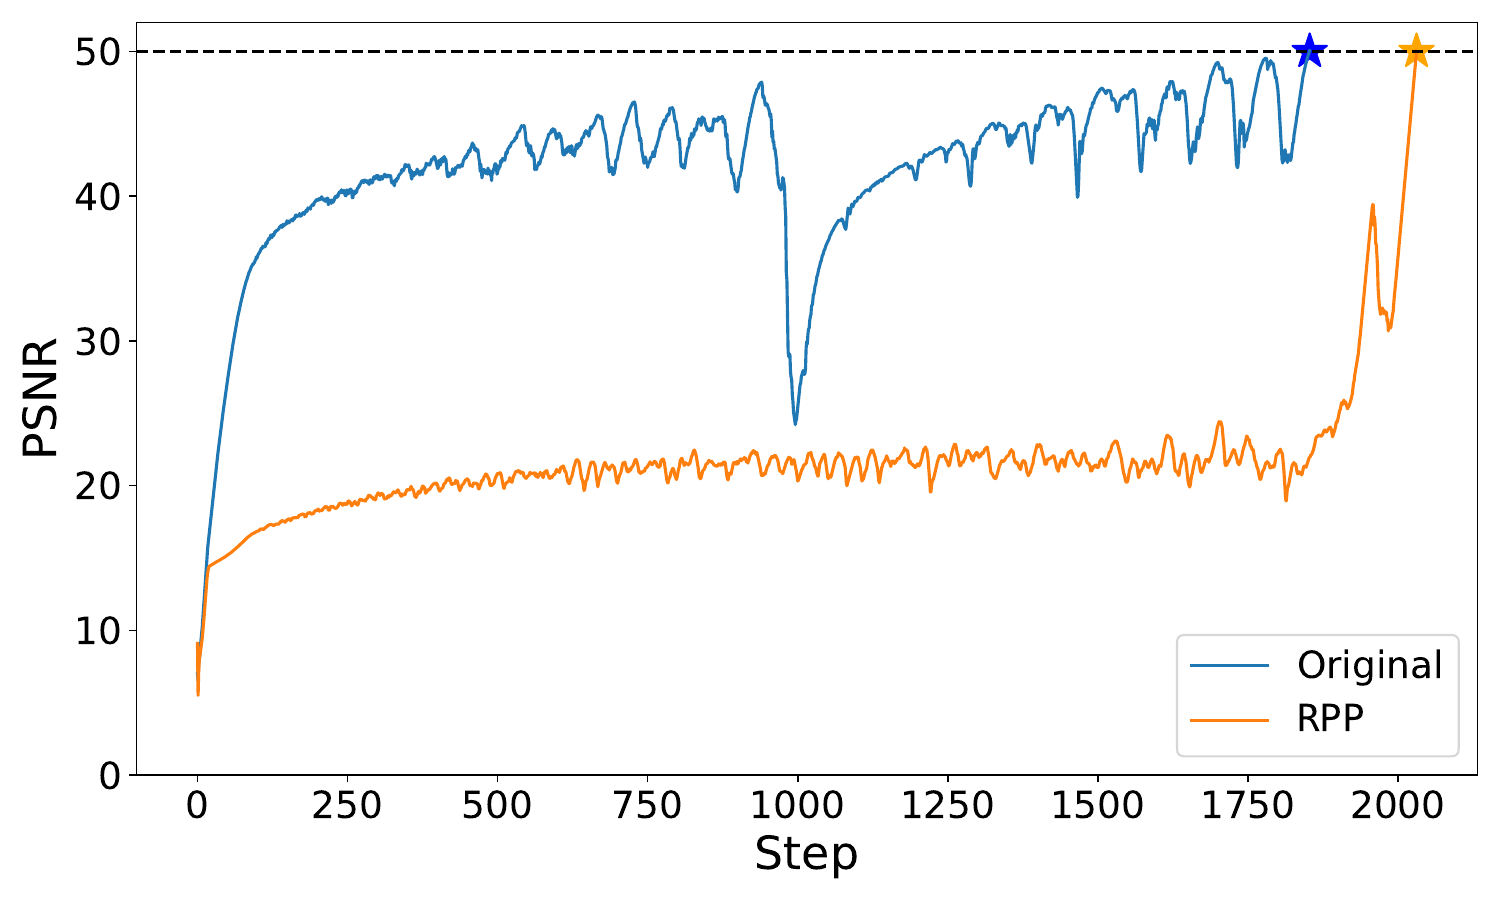}
        \captionsetup{skip=0pt}
        \caption{CLIC 03}
        \label{fig:lc_clic3}
    \end{subfigure}
    
    % Row 2
    \vspace{0.1cm}
    \begin{subfigure}[t]{0.32\linewidth}
        \centering
        \includegraphics[width=\linewidth]{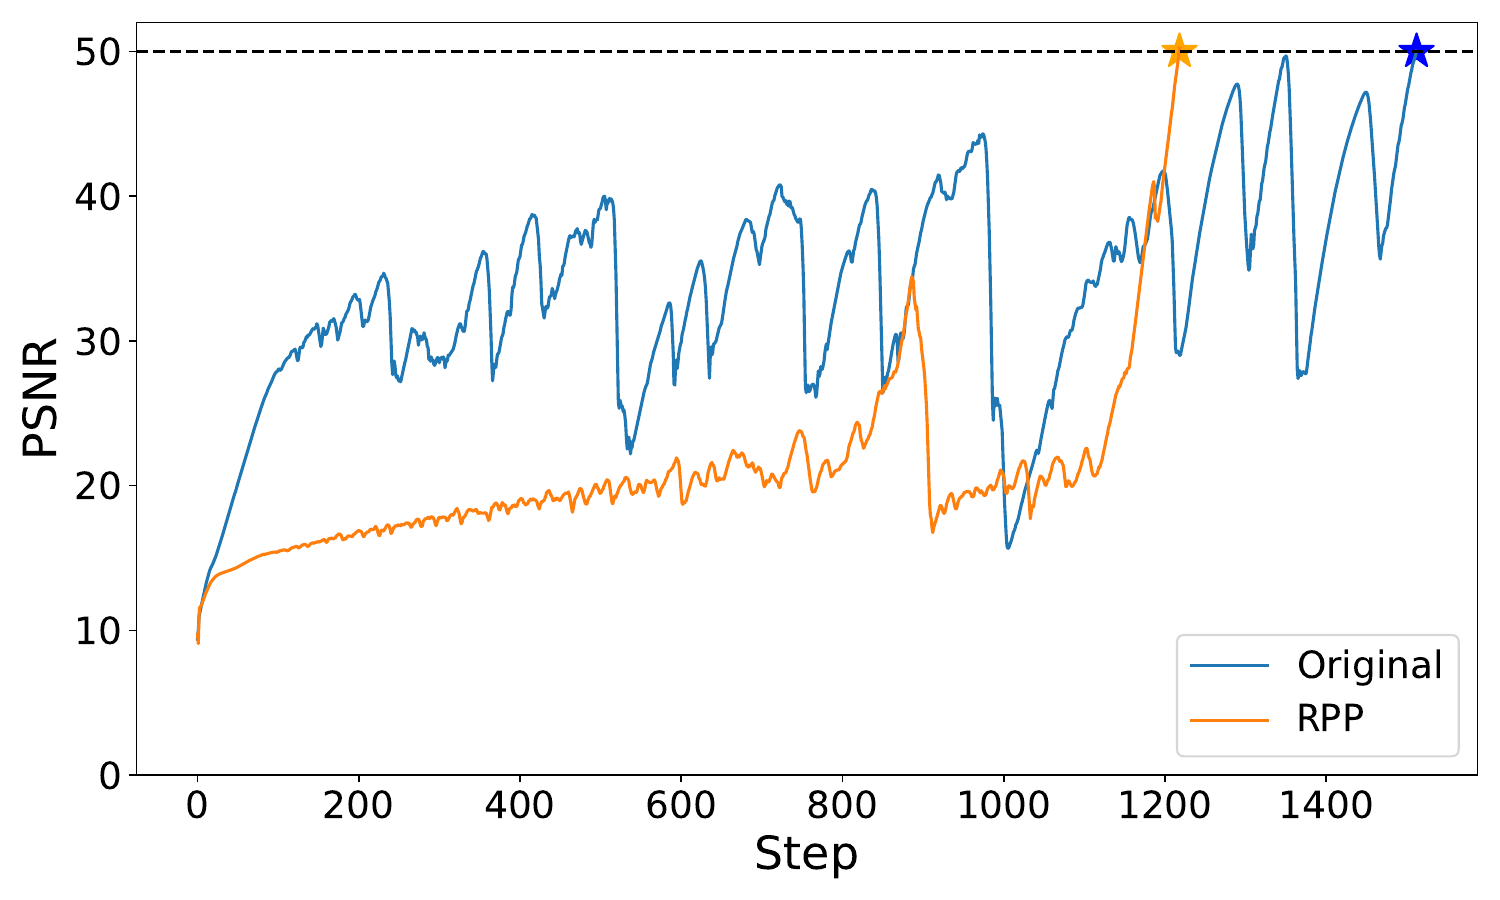}
        \captionsetup{skip=0pt}
        \caption{CLIC 04}
        \label{fig:lc_clic4}
    \end{subfigure}
    \hfill
    \begin{subfigure}[t]{0.32\linewidth}
        \centering
        \includegraphics[width=\linewidth]{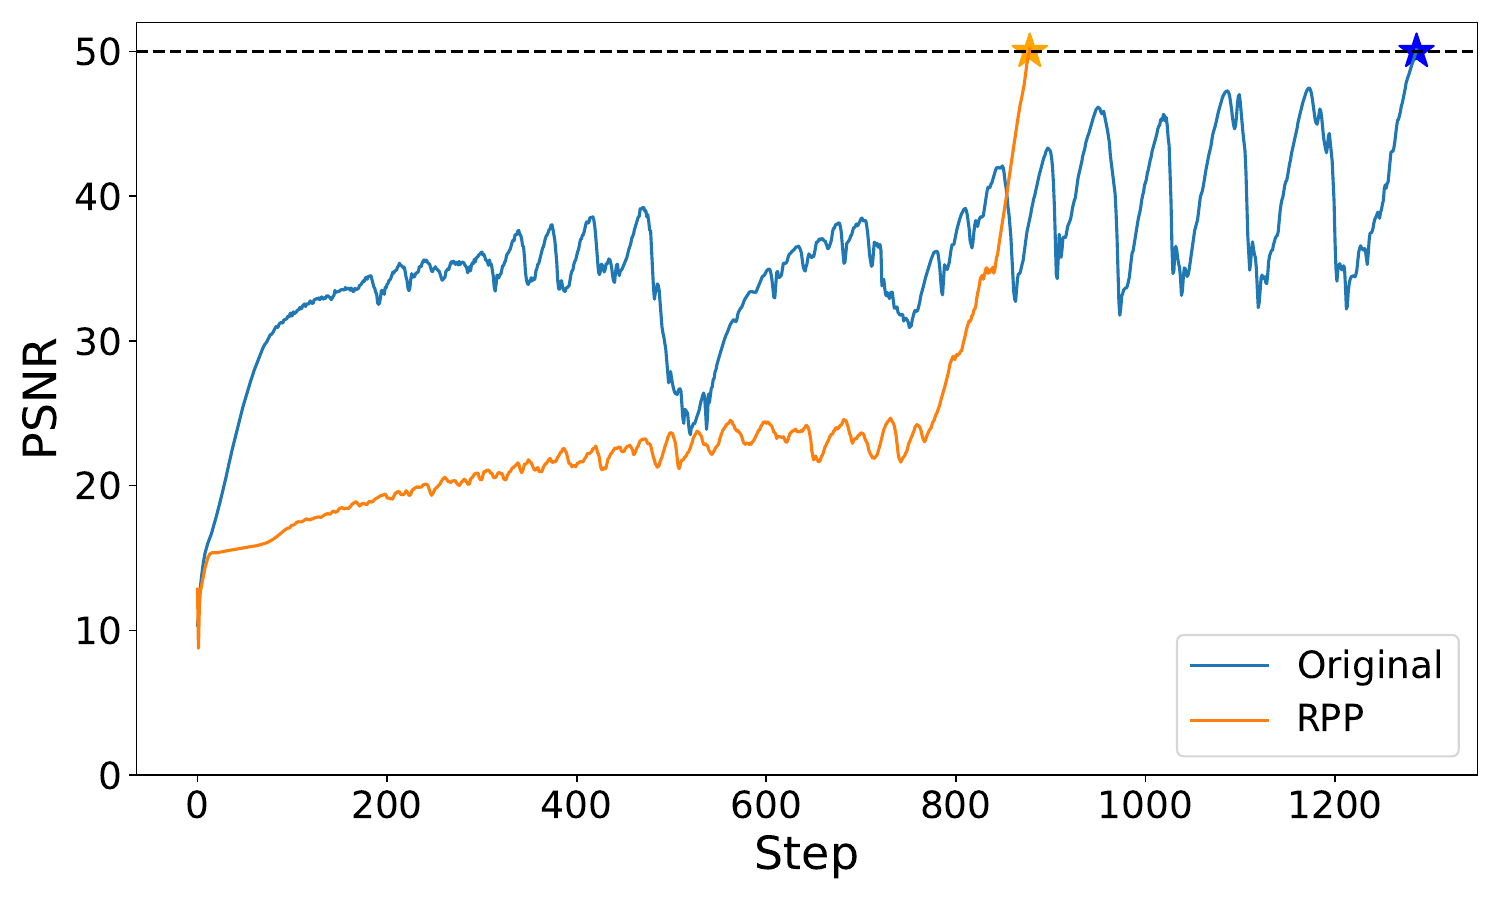}
        \captionsetup{skip=0pt}
        \caption{CLIC 05}
        \label{fig:lc_clic5}
    \end{subfigure}
    \hfill
    \begin{subfigure}[t]{0.32\linewidth}
        \centering
        \includegraphics[width=\linewidth]{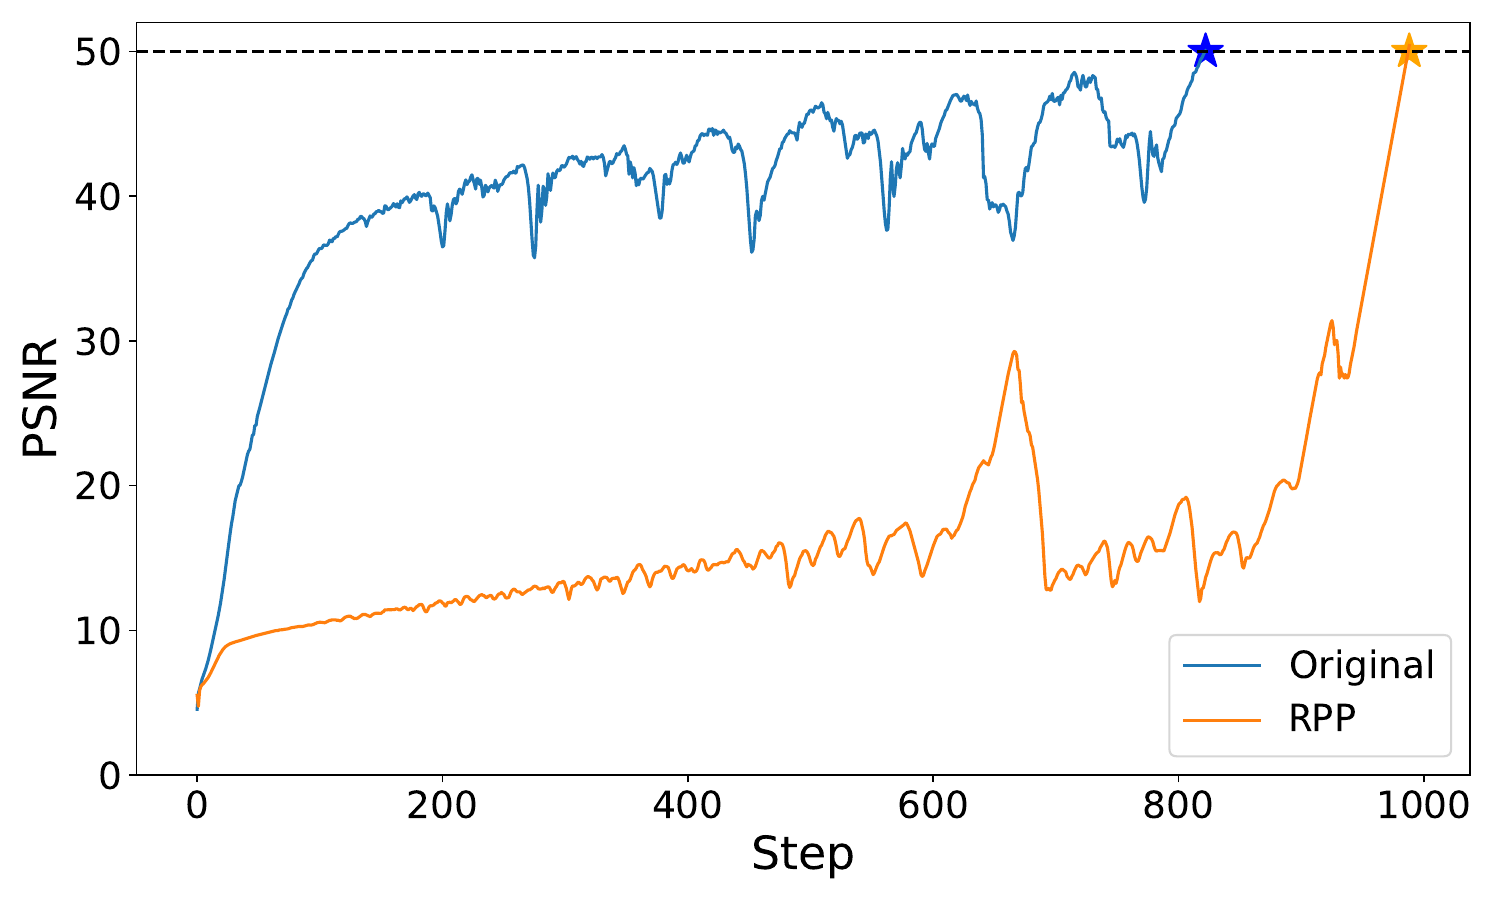}
        \captionsetup{skip=0pt}
        \caption{CLIC 06}
        \label{fig:lc_clic6}
    \end{subfigure}

    % Row 3
    \vspace{0.1cm}
    \begin{subfigure}[t]{0.32\linewidth}
        \centering
        \includegraphics[width=\linewidth]{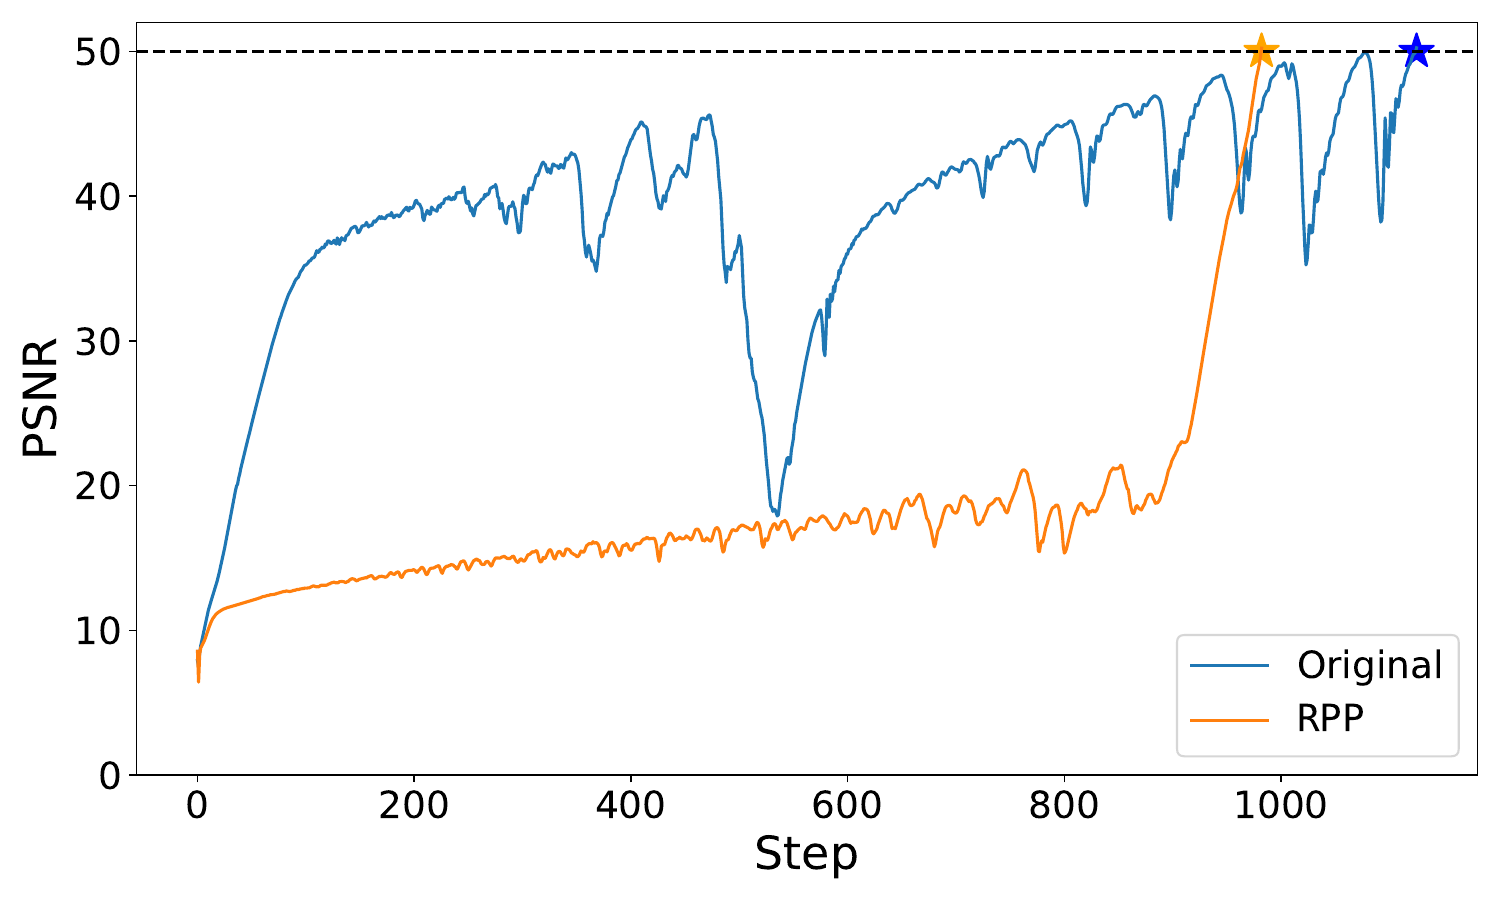}
        \captionsetup{skip=0pt}
        \caption{CLIC 07}
        \label{fig:lc_clic7}
    \end{subfigure}
    \hfill
    \begin{subfigure}[t]{0.32\linewidth}
        \centering
        \includegraphics[width=\linewidth]{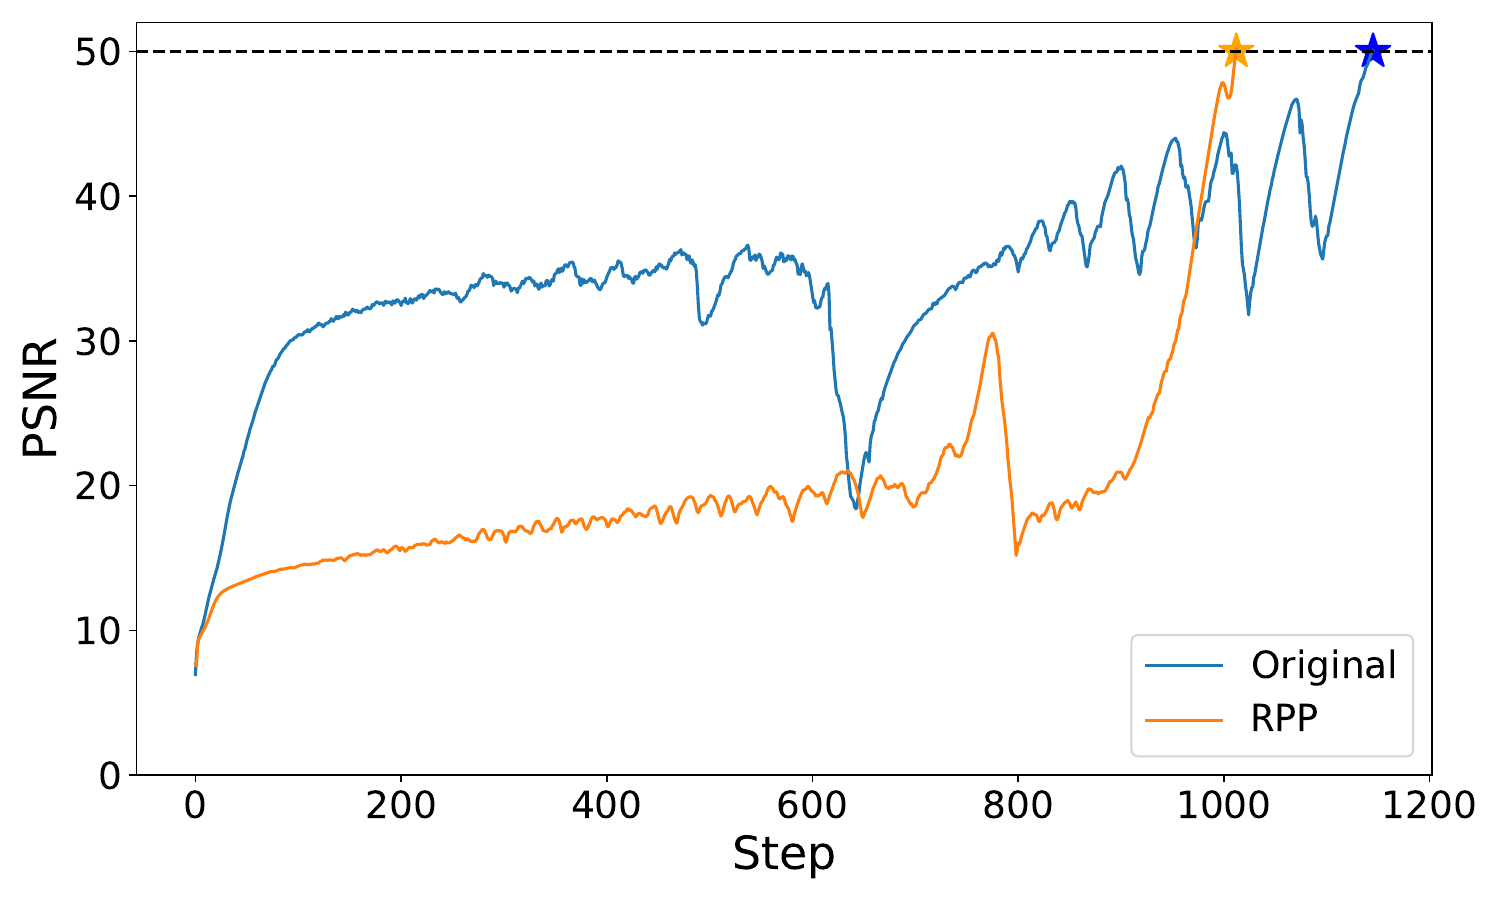}
        \captionsetup{skip=0pt}
        \caption{CLIC 08}
        \label{fig:lc_clic8}
    \end{subfigure}
    \hfill
    \begin{subfigure}[t]{0.32\linewidth}
        \centering
        \includegraphics[width=\linewidth]{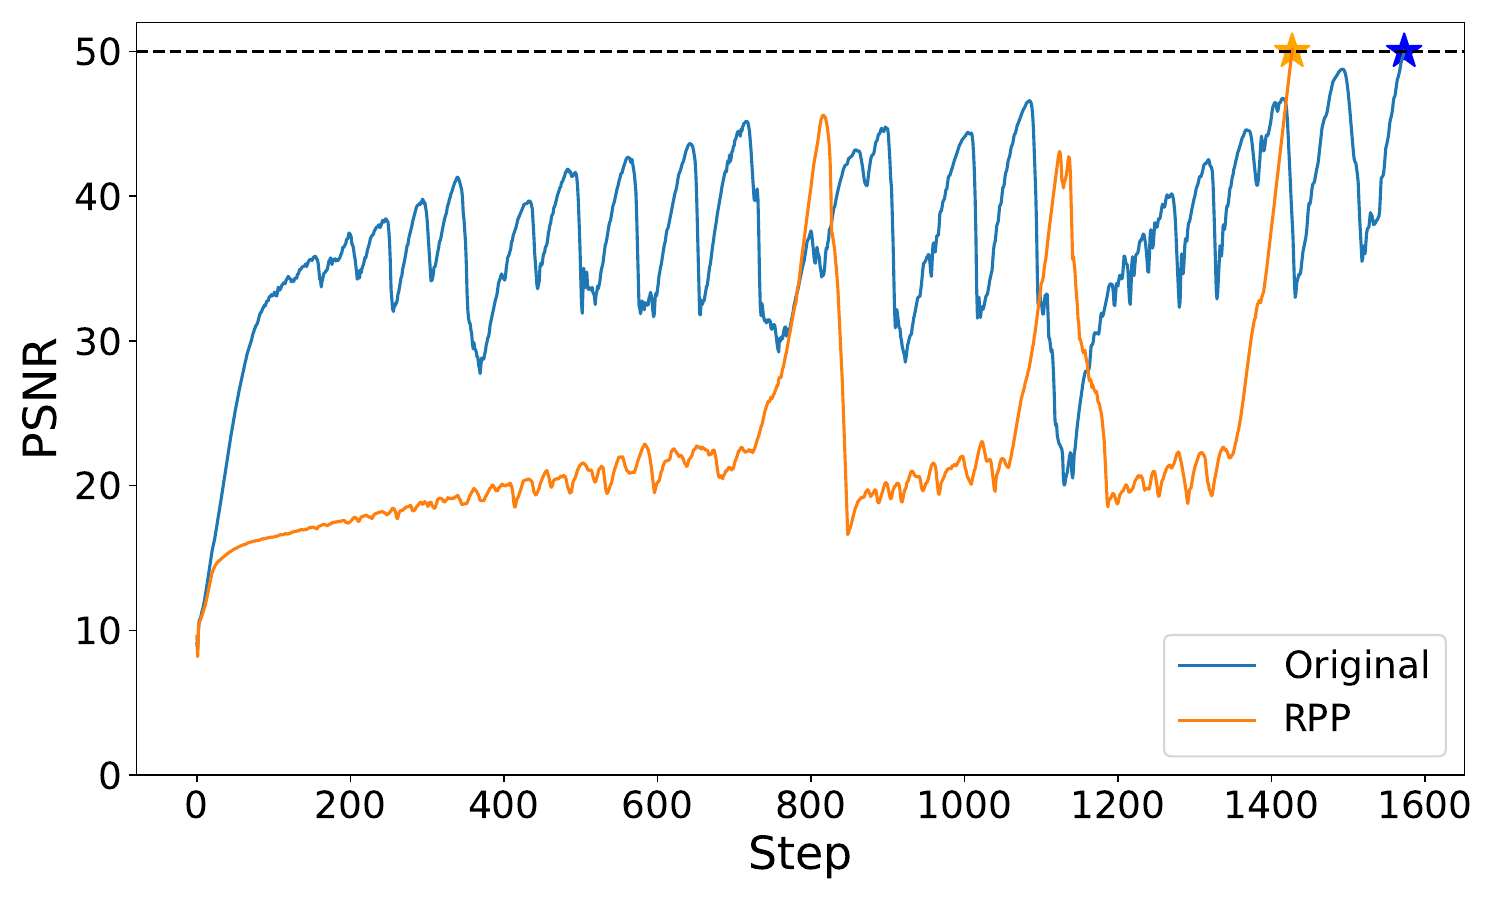}
        \captionsetup{skip=0pt}
        \caption{CLIC 09}
        \label{fig:lc_clic9}
    \end{subfigure}
    
    \caption{\textbf{PSNR Curves of CLIC images}}
    \label{fig:lc_clic}
    \vspace{-1em}
\end{figure*}
