# Supplementary material for: In Search of a Data Transformation That Accelerates Neural Field Training
Source: arXiv:2311.17094 source file (2024-03-26)
Supplement: Supplementary file 2 [file LC_div2k.tex]

\begin{figure*}[!t]
\centering
    % Row 1
    \begin{subfigure}[t]{0.32\linewidth}
        \centering
        \includegraphics[width=\linewidth]{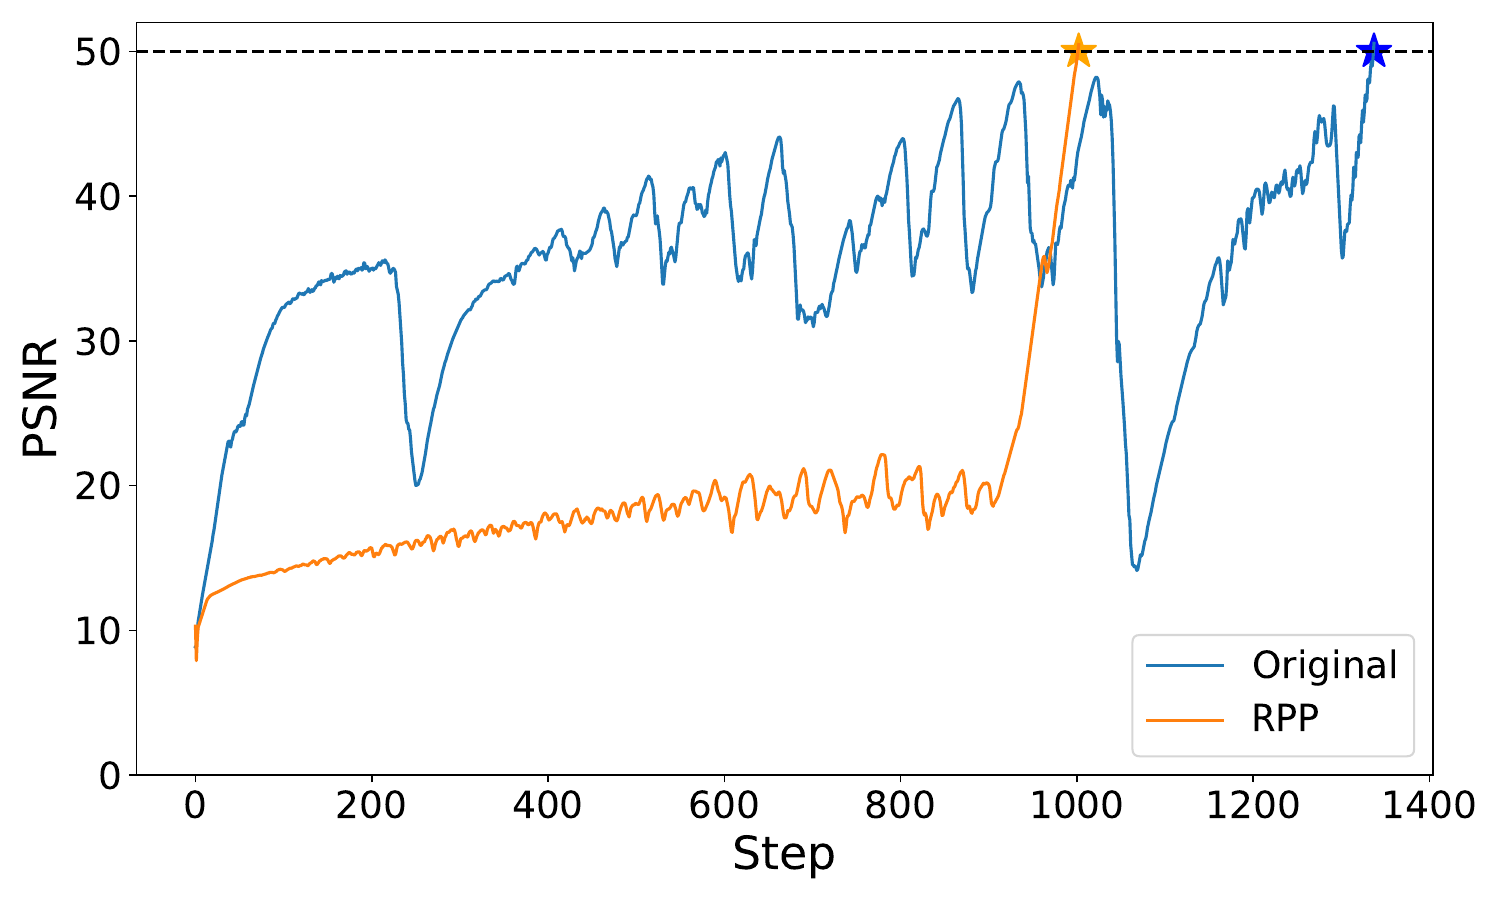}
        \captionsetup{skip=0pt}
        \caption{DIV2K 801}
        \label{fig:lc_div2k1}
    \end{subfigure}
    \hfill
    \begin{subfigure}[t]{0.32\linewidth}
        \centering
        \includegraphics[width=\linewidth]{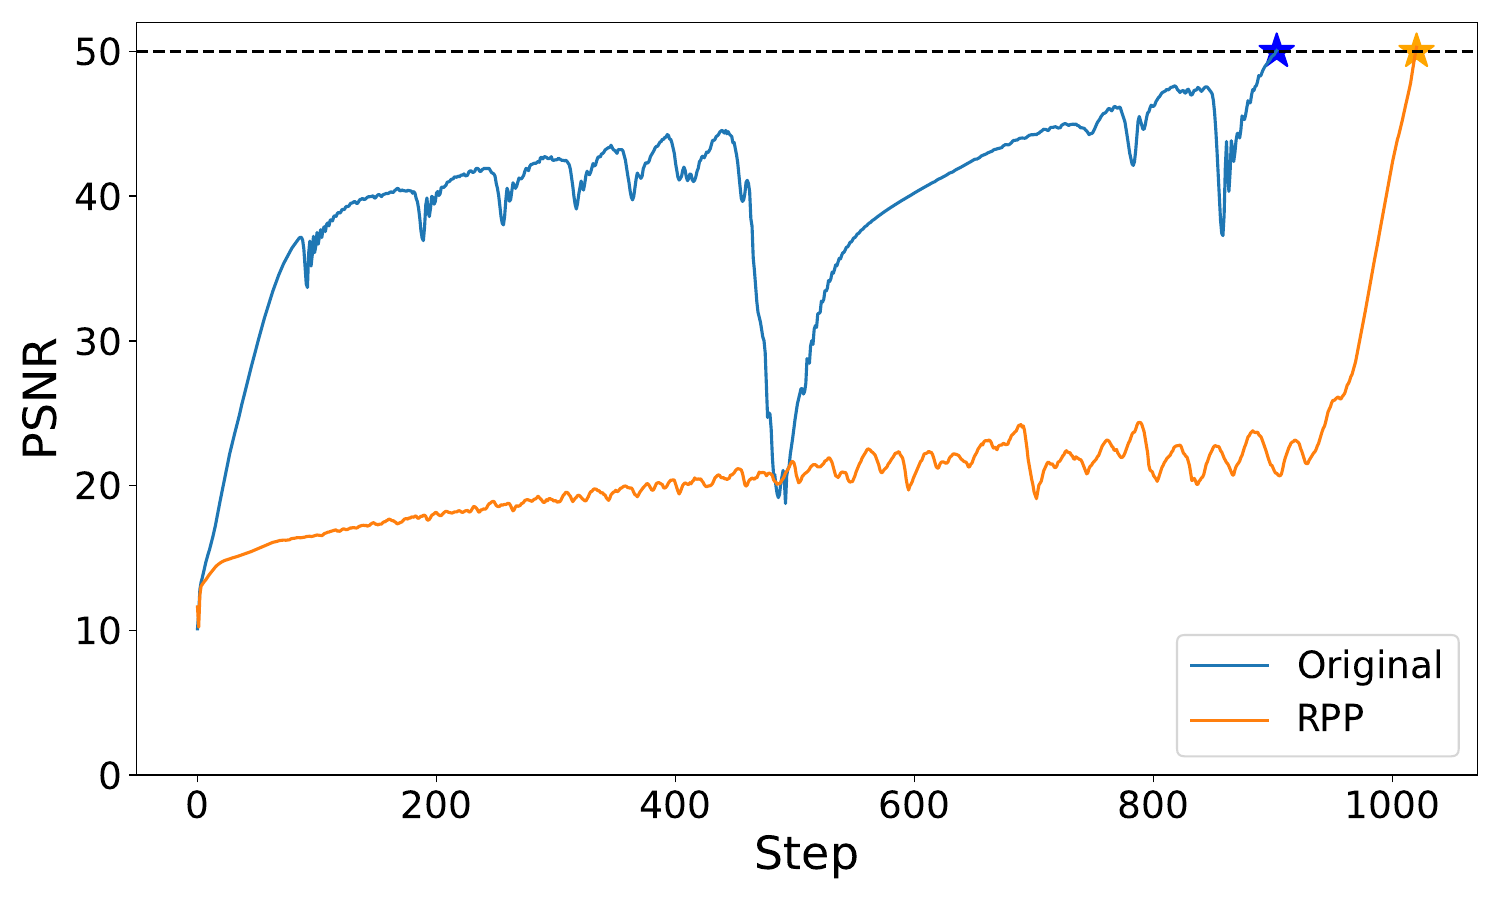}
        \captionsetup{skip=0pt}
        \caption{DIV2K 802}
        \label{fig:lc_div2k2}
    \end{subfigure}
    \hfill
    \begin{subfigure}[t]{0.32\linewidth}
        \centering
        \includegraphics[width=\linewidth]{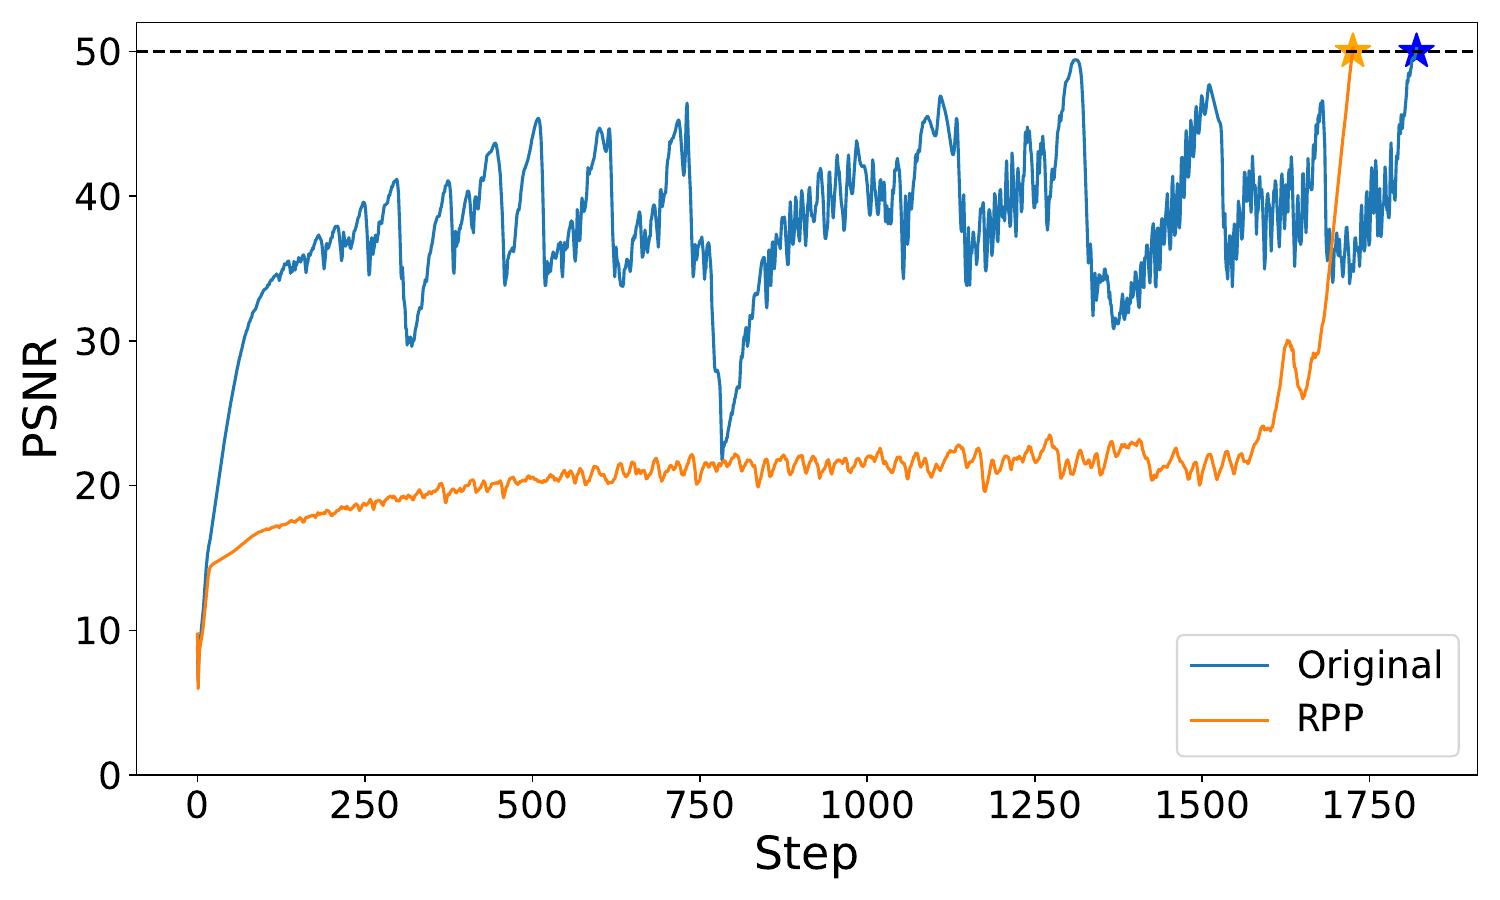}
        \captionsetup{skip=0pt}
        \caption{DIV2K 803}
        \label{fig:lc_div2k3}
    \end{subfigure}
    
    % Row 2
    \vspace{0.1cm}
    \begin{subfigure}[t]{0.32\linewidth}
        \centering
        \includegraphics[width=\linewidth]{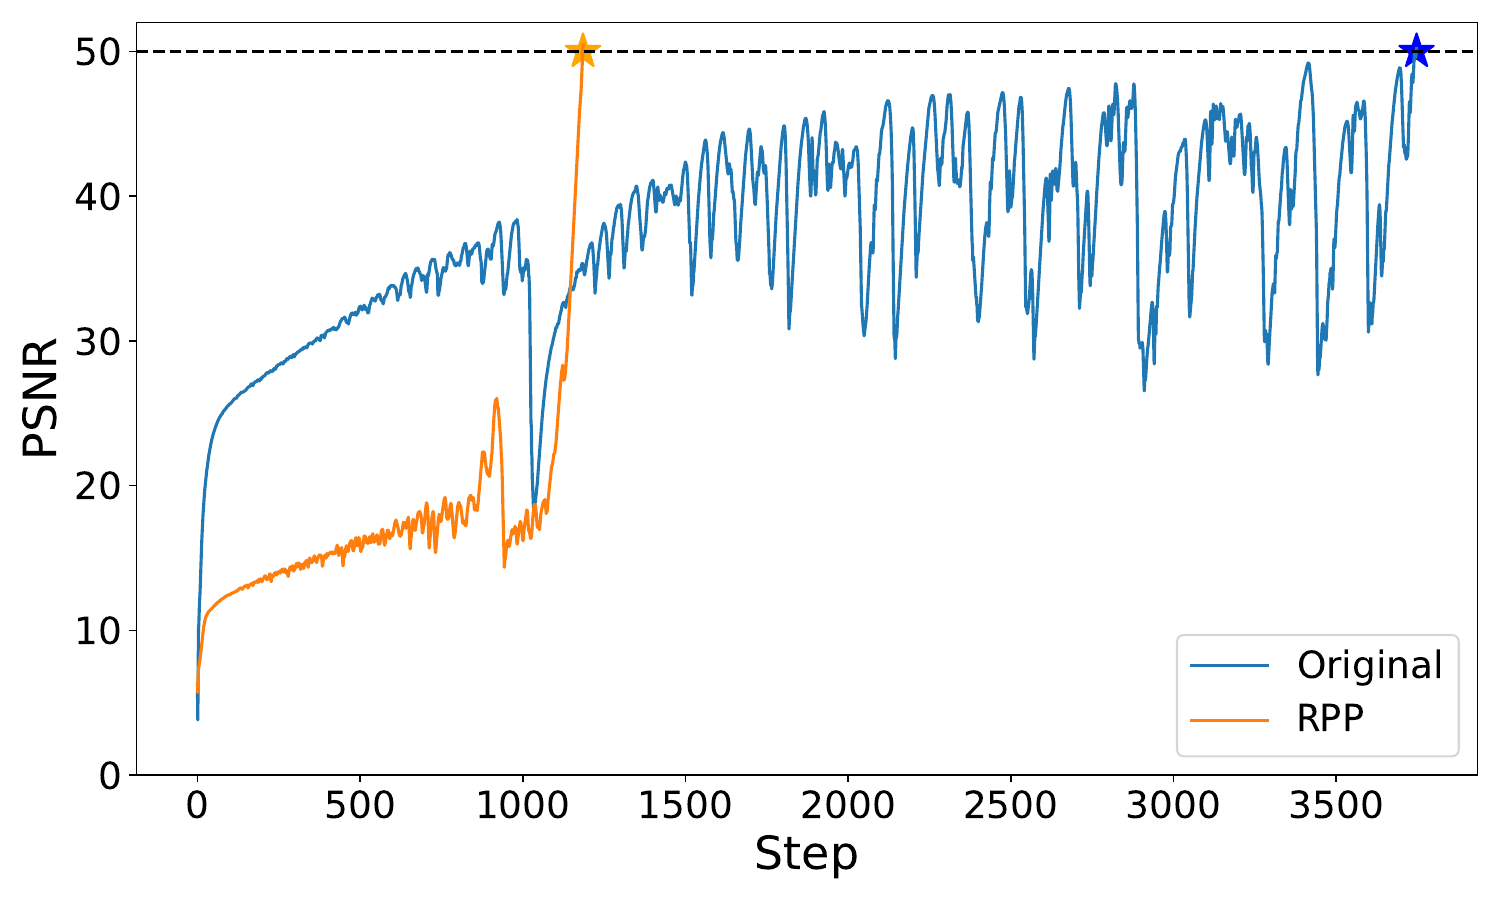}
        \captionsetup{skip=0pt}
        \caption{DIV2K 804}
        \label{fig:lc_div2k4}
    \end{subfigure}
    \hfill
    \begin{subfigure}[t]{0.32\linewidth}
        \centering
        \includegraphics[width=\linewidth]{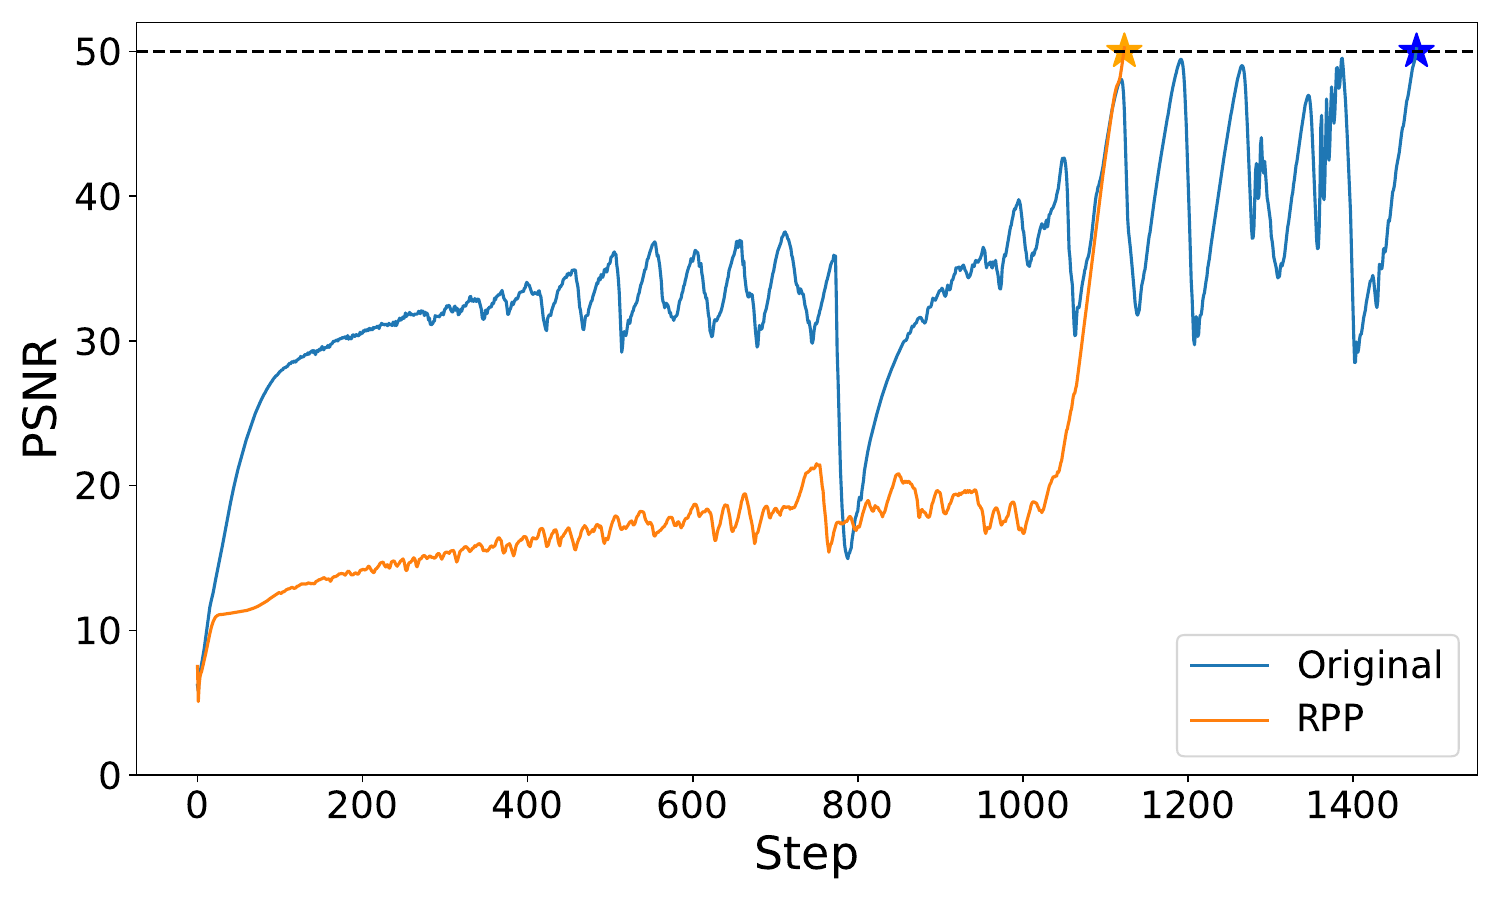}
        \captionsetup{skip=0pt}
        \caption{DIV2K 805}
        \label{fig:lc_div2k5}
    \end{subfigure}
    \hfill
    \begin{subfigure}[t]{0.32\linewidth}
        \centering
        \includegraphics[width=\linewidth]{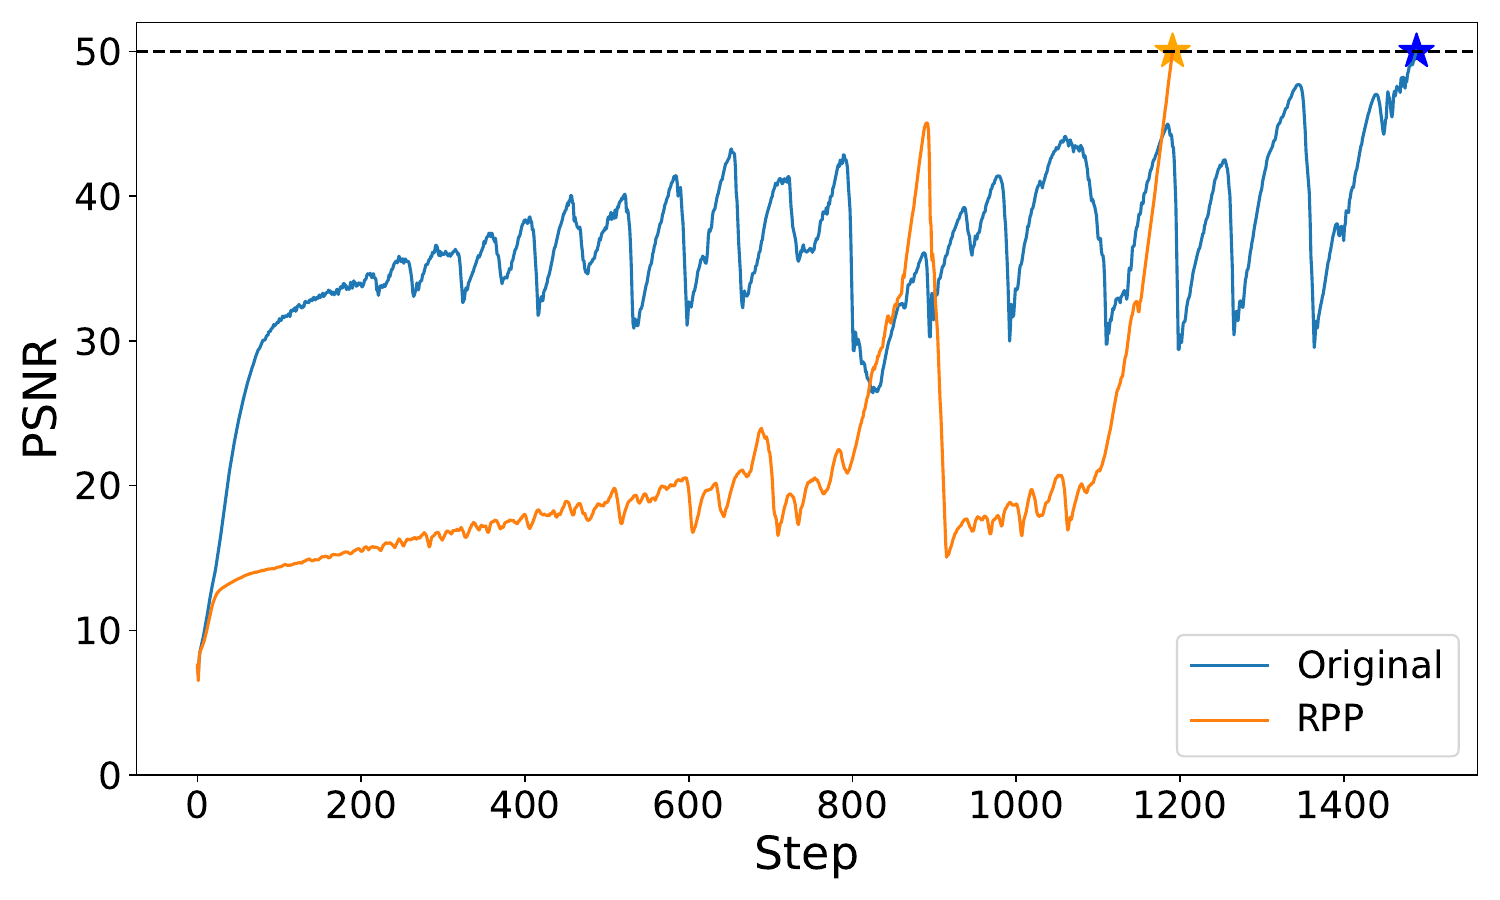}
        \captionsetup{skip=0pt}
        \caption{DIV2K 806}
        \label{fig:lc_div2k6}
    \end{subfigure}

    % Row 3
    \vspace{0.1cm}
    \begin{subfigure}[t]{0.32\linewidth}
        \centering
        \includegraphics[width=\linewidth]{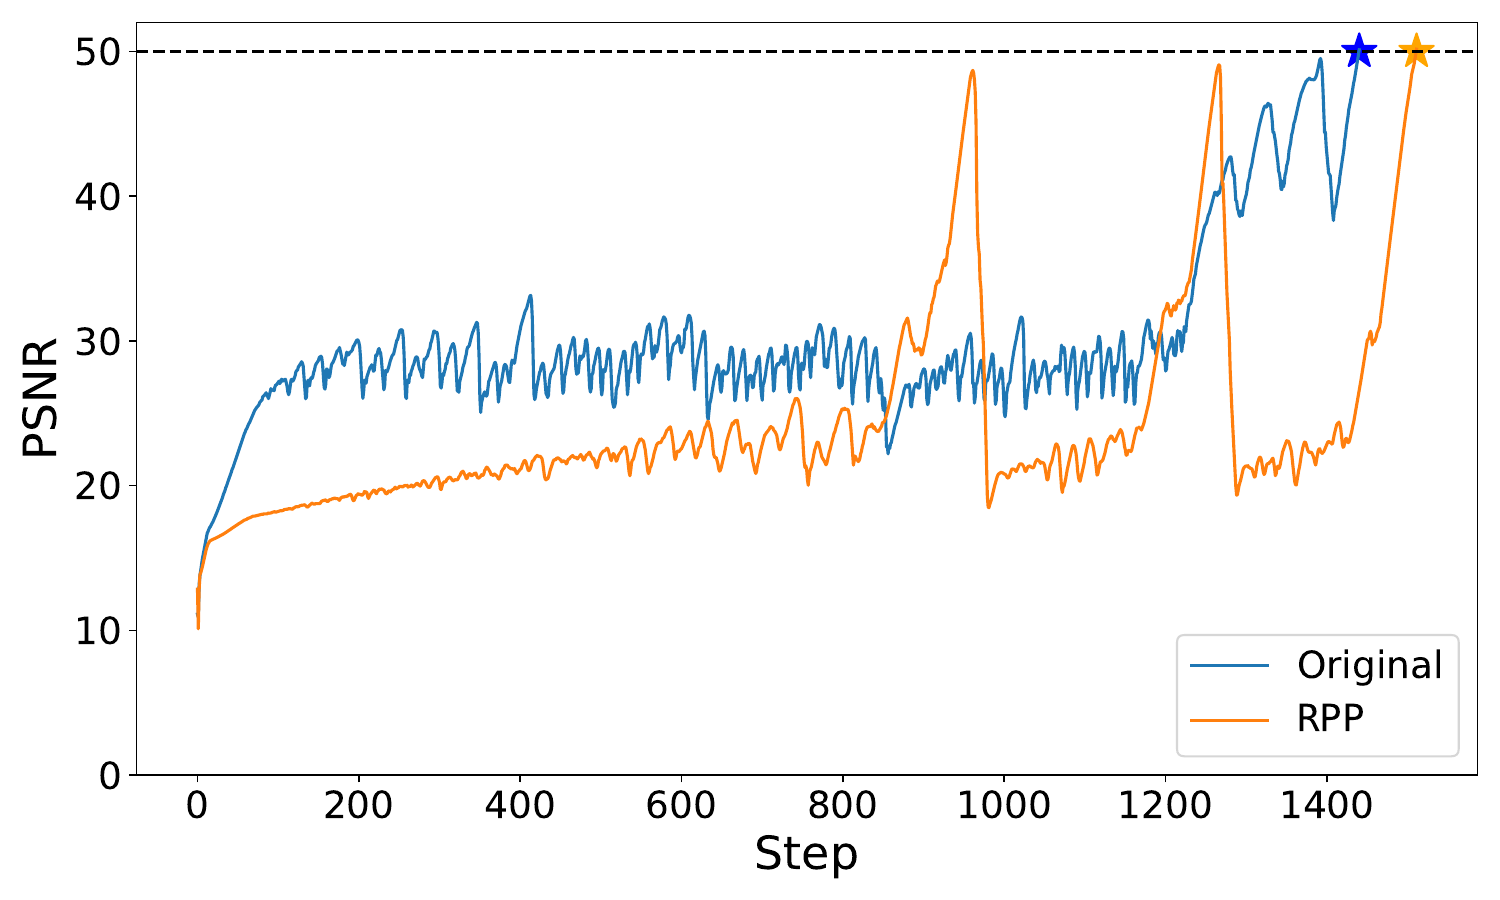}
        \captionsetup{skip=0pt}
        \caption{DIV2K 807}
        \label{fig:lc_div2k7}
    \end{subfigure}
    \hfill
    \begin{subfigure}[t]{0.32\linewidth}
        \centering
        \includegraphics[width=\linewidth]{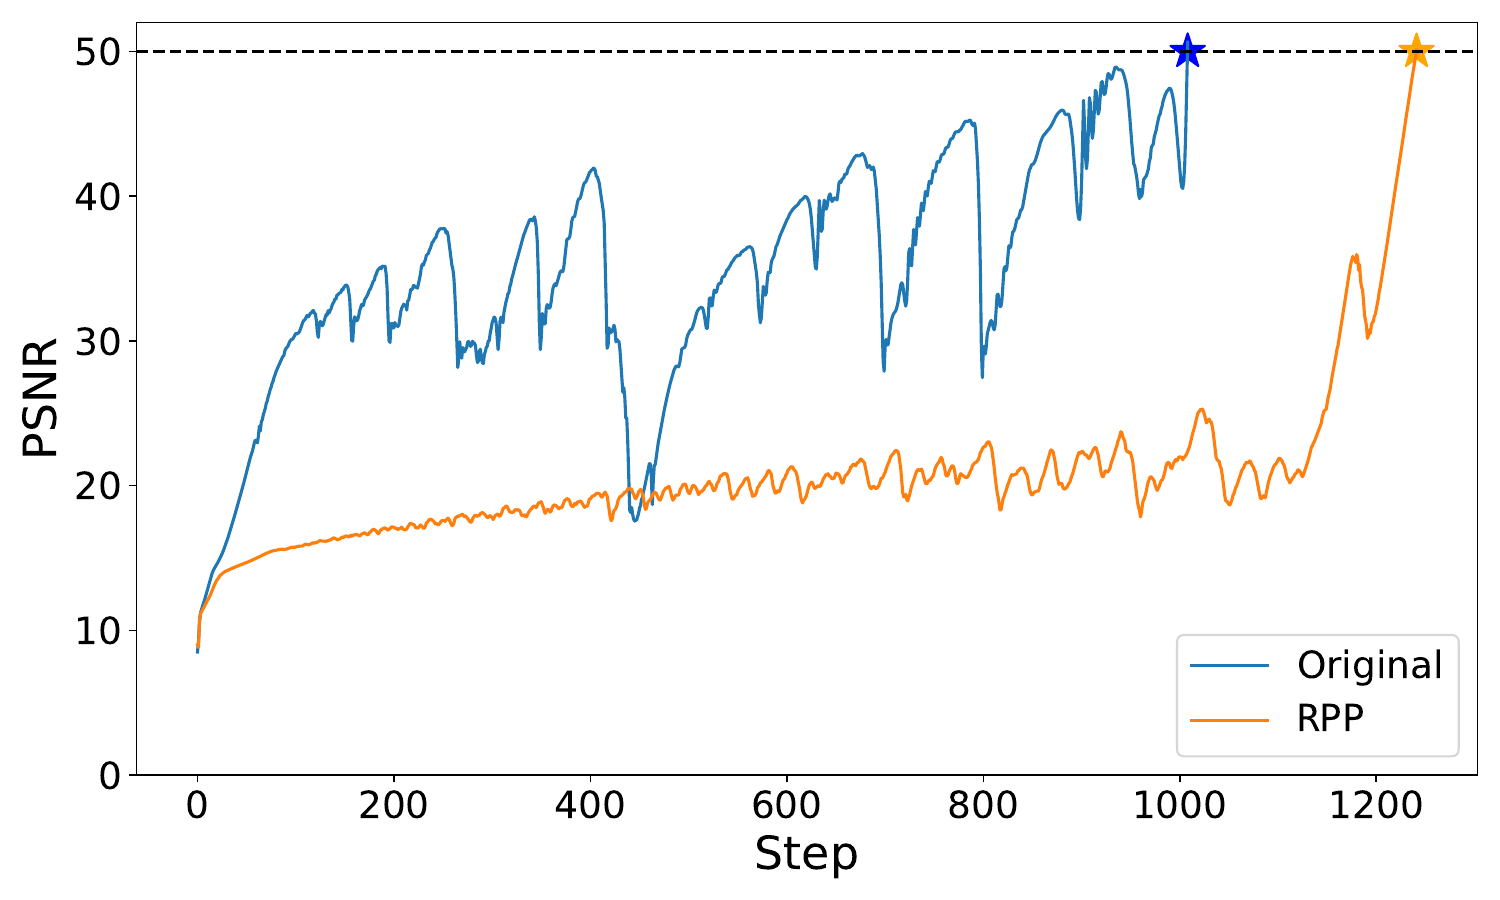}
        \captionsetup{skip=0pt}
        \caption{DIV2K 808}
        \label{fig:lc_div2k8}
    \end{subfigure}
    \hfill
    \begin{subfigure}[t]{0.32\linewidth}
        \centering
        \includegraphics[width=\linewidth]{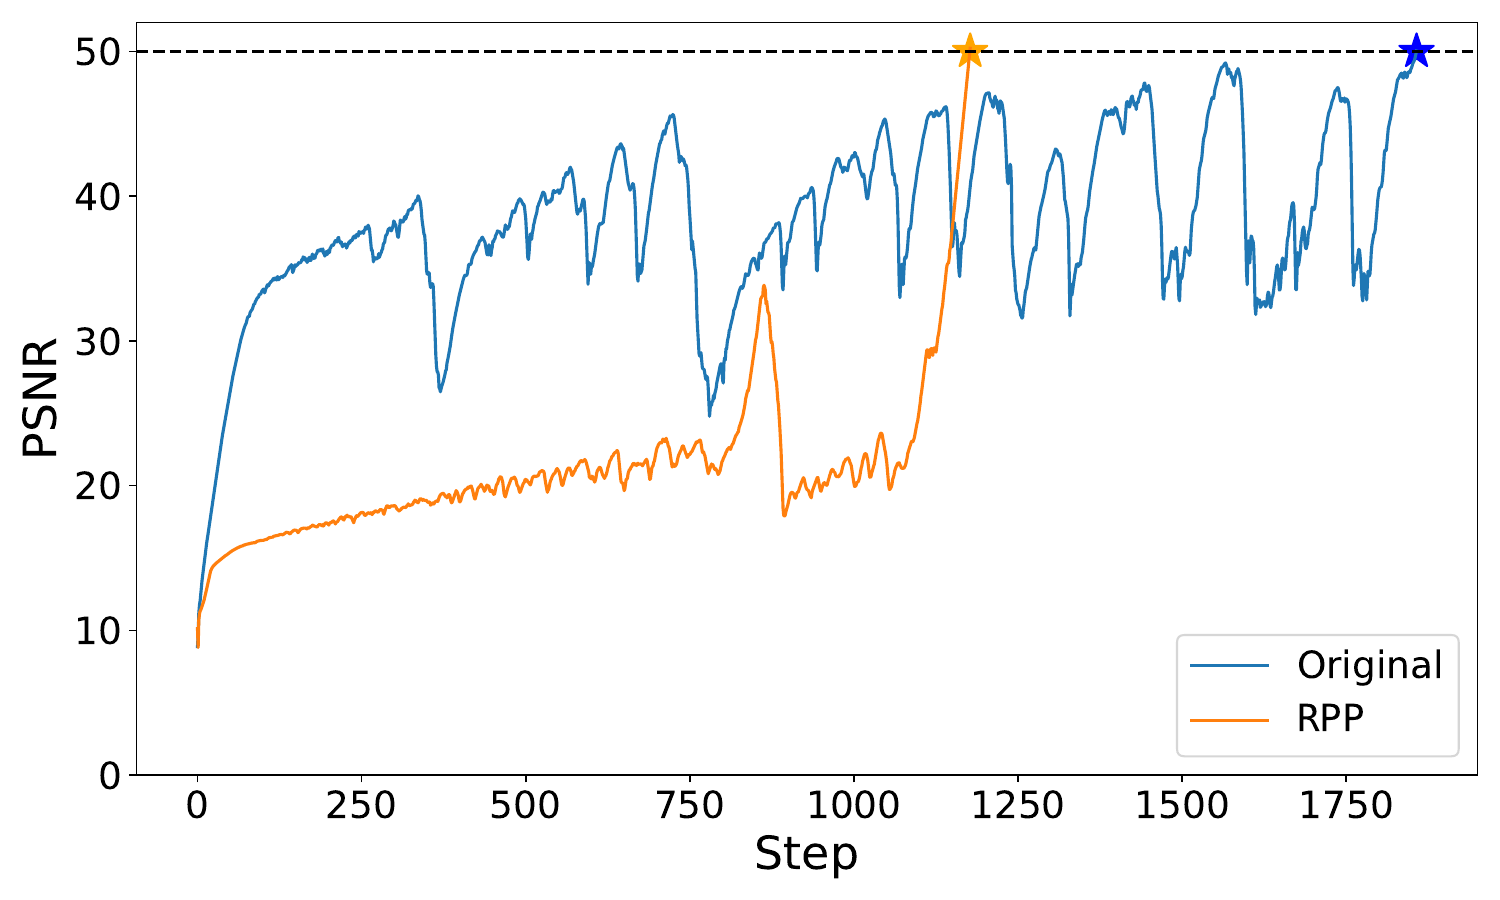}
        \captionsetup{skip=0pt}
        \caption{DIV2K 809}
        \label{fig:lc_div2k9}
    \end{subfigure}
    
    \caption{\textbf{PSNR Curves of DIV2K images}}
    \label{fig:lc_div2k}
    \vspace{-1em}
\end{figure*}
